# Supplementary material for: TaRL: Learning General and Physical Rewards from Tactile Demonstrations
Source: arXiv:2609.36785 source file (2026-09-29)
Supplement: Supplementary file 1 [file 7_appendix.tex]

\section*{Experiment Details}
\label{sec:appendix_experiment_details}
In this section, we detail the training configuration and experiment setup used in our experiments.
For all experiments, we build on the Isaac Lab Forge contact-rich manipulation
suite and train policies with PPO using the \texttt{rl\_games}
implementation. Unless otherwise stated, all baselines and our method share the
identical PPO optimizer, network architecture, and environment configuration
summarized in Table~\ref{tab:training_hyperparameters}; they differ only in the
observation composition and the reward formulation.

% \paragraph{Tasks.}
% We evaluate on three contact-rich pick-and-place insertion tasks built on the
% Forge environment: \emph{peg-insert}, \emph{gear-mesh}, and \emph{nut-thread}.
% Each task is a long-horizon variant requiring the agent to grasp the held object
% at a source location, lift and transport it, and precisely insert it into a
% destination hole. The destination and source poses are randomized at every reset.
% Episodes run for $20$ simulation seconds. With a physics timestep of $1/120$\,s
% and a control decimation of $8$, this corresponds to an episode length of $300$ policy steps. The action space is
% $8$-dimensional: a $6$-DoF relative pose target, a learned success-prediction
% output, and a gripper command. We run $256$ parallel environments for training.
\paragraph{Tasks.}
We evaluate on three contact-rich assembly tasks: Peg Insertion,
Gear Assembly, and Nut Threading.  These are the three canonical tasks from
the Forge benchmark, in which a
Franka arm manipulates a \emph{held asset}, grasped in the gripper for intialization, and a
\emph{fixed asset} mounted on the table. In the original formulation, each
episode begins with the held asset \emph{already grasped} and positioned directly
above the fixed asset with a small pose perturbation; the agent only has to
perform the final alignment and insertion. Concretely: 
\begin{itemize}
  \item \textbf{Peg Insertion.} An $8$\,mm cylindrical peg be inserted
    into a tight-clearance socket; success requires the peg to bottom out
    in the socket.
  \item \textbf{Gear Assembly.} A medium gear be lowered onto the central
    shaft of a gear base so that its teeth mesh with the pre-placed small
    and large gears, demanding precise rotational and translational alignment.
  \item \textbf{Nut Threading.} An M16 nut be threaded onto an M16 bolt. Beyond positional alignment, this task requires the agent to rotate
    the nut to engage the thread and screw it down, making it the
    most contact-rich and longest-horizon of the three; success requires reaching $30\%$ of the thread height.
\end{itemize}
The original tasks isolate the insertion skill: the object is pre-grasped, the
gripper is held closed, and the action space is the $6$-DoF end-effector pose
target.

We extend each of these into a long-horizon \emph{pick-and-place} variant that
also requires grasping and transport. At reset, the asset is placed
at a \emph{source} location roughly $10$\,cm
away from the target fixture, and the gripper starts open above it. The agent
must therefore (1) approach and grasp the object at the source location, (2) lift it above the source location, (3) transport it to the target fixture, and (4) align and
insert or thread it into the target fixture. Both the initial asset pose and target fixture pose
are randomized independently at every reset, subject to a minimum centre-to-centre distance so they never overlap. To support grasping and a learned termination
signal, we expand the action space to $8$ dimensions: a $6$-DoF relative pose
target, a binary gripper command, and a learned success-prediction output. This
turns each task from a short-horizon insertion problem into a full grasp\,$\to$\,
lift\,$\to$\,transport\,$\to$\,insert sequence, substantially increasing the
horizon and the reliance on robust contact during grasping and insertion.



\paragraph{Policy and value architecture.}
We train the policy with PPO in an actor-critic setup. Both the actor and the asymmetric critic share an LSTM core of $1024$ units with $2$ layers followed by an MLP with hidden sizes $[512, 128, 64]$ and ELU activations. The critic is trained with privileged state information that is withheld from the actor. We use a fixed action standard deviation ($\log\sigma = 0$, i.e.\ $\sigma = 1$) to prevent the policy from prematurely collapsing exploration once it discovers a local optimum. Inputs, values, and advantages are normalized, and we use value bootstrapping on
truncated episodes. Full PPO and network hyperparameters are listed in
Table~\ref{tab:training_hyperparameters}.

\paragraph{Reward shaping.}
We introduce multiple reward terms, excluding contact rewards, which enable us to succeed the task. Specifically, we use a reward that encourages the end-effector approaching the source location, a reward that encourages lifting the asset, a reward that encourages relocating the asset at the XY target location, and a reward that encourages putting down the asset.  With these rewards, the baseline solves the task eventually with a large number of interaction steps without any contact information.


\input{src/tab_training_hyperparameter}

\section*{Tactile pattern analysis}
\label{sec:appendix_tactile_pattern}

To further verify whether tactile signals provide useful information for distinguishing tasks that cannot be obtained from vision or proprioception alone, we project
the tactile trajectory of all four manipulation tasks
(Peg Insertion, Gear Assembly, Nut Threading, and
Box Placement) into a shared 2D space and inspect their separability.
\paragraph{Per-trajectory feature.}
Each trajectory $\tau$ provides a per-finger tactile tensor of shape
$(T, 20, 25, 3)$ for each of the two parallel-jaw fingers, recorded by the
fingertip tactile sensors. For each taxel, we summarize the tactile signal over time using the peak force
magnitudes along the three axes and the fraction of timesteps with nonzero
contact:
\[
  \phi(\tau)_{ij}
  =
  \left(
    \max_t |f_{x,t}|,\;
    \max_t |f_{y,t}|,\;
    \max_t |f_{z,t}|,\;
    \frac{1}{T}\sum_t \mathbf{1}\!\left[\|\mathbf{f}_t\| > 0\right]
  \right).
\]
We compute this four-channel descriptor over the $20 \times 25$ taxel grid for
each finger and concatenate the descriptors from both fingers. This yields a
$4000$-dimensional feature vector for each trajectory, capturing where contact
occurs, the maximum force magnitude along each axis, and how persistently each
taxel remains in contact.

\paragraph{Projection.}
We standardize the resulting feature matrix to have zero mean and unit variance
in each dimension. We then reduce the features to $50$ principal components
using PCA and project them to two dimensions with t-SNE, using perplexity $30$,
PCA initialization, and the automatic learning-rate setting.


\paragraph{Tactile signals distinguish task identities.}
Figure~\ref{fig:tactile_tsne} shows that successful trajectories of the four tasks
form clearly separated clusters in the projected space. This indicates that the raw tactile signal alone is sufficient to identify the task and supports its use as a strong conditioning input to the policy.

\input{src/fig_tsne_tactile}

\section*{Task Generalization}
\label{sec:appendix_task_generalize}
In this section, we examine
whether tactile pattern contains enough information that a reward model trained
\emph{only} on one task can transfer directly to the other in a zero-shot
manner.

\paragraph{Cross-task evaluation protocol.}
For each source task $s \in \{\textsc{peg}, \textsc{gear}, \textsc{nut}, \textsc{box}\}$,
we take the reward model trained on $s$ and apply it, without any
fine-tuning, to trajectories collected from every other task $t \neq s$.
We follow the same evaluation protocol as Section~3.1, measuring the
reward gap between successful and failed trajectories under both
in-domain and out-of-distribution settings.

\paragraph{Generalization across tasks.}
As shown in Figure~\ref{fig:cross_task_grid} (middle of the second row), the Gear Assembly reward model achieves $\Delta_{\text{ID}} = +0.132$ and $\Delta_{\text{OOD}} = +0.141$ when evaluated directly on Nut Threading tactile trajectories, consistent with the observation in Section~\ref{sec:appendix_tactile_pattern}, indicating that the shared rotational contact signature between the two tasks is informative enough for the reward model to rank successful and failed trajectories correctly without ever observing the target task during training. Importantly, the positive gap persists under the OOD multi-position split, suggesting that
the model keys on the underlying contact dynamics rather than memorizing task-specific spatial cues.

Notably, the reward models trained on Gear Assembly and Nut Threading are both able to distinguish tactile trajectories from Box Placement, as both tasks involve steadily grasping a similarly shaped object before performing their own contact-rich manipulation. This shared grasping phase provides a common tactile prefix that the reward model can latch onto, even when the subsequent manipulation differs. In contrast, source models trained on Peg Insertion transfer poorly to the other tasks, the predicted-reward curves remain low and largely overlapping between success and failure trajectories, reflecting the absence of a comparable shared contact signature. We also observe that generalization is not symmetric: the strength of transfer depends on the direction of the source--target pair, which we attribute to differences in the richness and discriminability of each task's contact phase.

Taken together, these results indicate that \method{} generalizes not
only across different objects but also across different manipulation
tasks, provided the tasks share an underlying contact structure. This
supports our central claim that tactile force fields capture
task-agnostic interaction dynamics, offering a transferable signal for reward shaping that purely visual reward models, which rely on
task-specific appearance cues, are unlikely to provide.

\input{src/fig_task_generalization}

\section*{Reward Generalization to Unseen Object Positions}
\label{sec:appendix_visualization}
In this section, we measure the performance of generalization from the single training
position to multiple unseen object positions across all the four tasks. Figure~\ref{fig:visual_tactile_viz} visualizes the predicted reward along successful rollouts for both the tactile and visual reward models for all four tasks, comparing the training position against positions held out during training. The tactile reward retains its performance of predicting monotonical reward at novel positions, whereas the visual reward degrades sharply, illustrating that tactile force fields capture position-invariant interaction dynamics that purely visual signals fail to provide.

\input{src/fig_visual_tactile_viz}
